# Supplementary material for: Text Matching Improves Sequential Recommendation by Reducing Popularity Biases
Source: arXiv:2308.14029 source file (2023-08-27)
Supplement: Supplementary file 1 [file appendix.tex]

\begin{appendix}
\begin{table}[t]
\begin{center}
\small
\resizebox{0.48\textwidth}{!}{
\begin{tabular}{l  r  r r r}
\hline \textbf{Dataset} & \textbf{Beauty} & \textbf{Yelp} & \textbf{Sports} & \textbf{Toys}\\ \hline
Users & 22,363 & 30,499 & 35,598 & 19,412   \\
Items & 12,101 & 20,068 & 18,357 & 11,924   \\
Interactions & 198,502 & 317,182 & 296,337 & 167,597   \\
Avg Item Length & 9 & 10 & 8 & 9   \\
Sparsity & 99.93\% & 99.95\% & 99.95\% & 99.93\%   \\ \hline
\end{tabular}}
\caption{\label{tab:dataset}Data Statistics of Yelp and Amazon Product. Amazon Product consists of Beauty, Sports, and Toys.}
\end{center}
\end{table}
\input{table/dataset.tex}
\begin{table*}[!ht]

\small
\begin{tabular}{p{0.2\linewidth}|p{0.7\linewidth}} 
\hline
\multicolumn{2}{l}{\textbf{Yelp}}
\tabularnewline 
\hline
User Interaction History & Here is the visit history list of user: id: 18078 title: Freed's Bakery address: 9815 S Eastern Ave Las Vegas NV, id: 650 title: Trattoria Italia address: 9905 S Eastern Ave, Ste 140 Las Vegas NV, id: 10540 title: Starbucks address: 3410 E Sunset Road Las Vegas NV, id: 16529 title: Starbucks address: 8975 S. Eastern Avenue, Las Vegas NV recommend next item
\tabularnewline 
\hline
Next Item & id: 6084 title: El Dorado Cantina address: 3025 Sammy Davis Jr Dr Las Vegas NV
\tabularnewline 
\hline

\multicolumn{2}{l}{\textbf{Beauty}}
\tabularnewline 
\hline
User Interaction History & Here is the visit history list of user: id: 8005 title: Neutrogena Ultra Gentle Soothing Lotion SPF 15, 4  Ounce, id: 451 title: GRANDPA'S BRANDS, Pine Tar Soap Bath Size - 4.25 oz, id: 29 title: Clean  Clear ESSENTIALS Dual Action Moisturizer, 4 Ounce, id: 34 title: Cetaphil Gentle Cleansing Bar, Antibacterial - 4.5 oz recommend next item
\tabularnewline 
\hline
Next Item & id: 6724 title: Head Shoulders Clinical Strength Dandruff Shampoo 14.2 Fl Oz (Pack of 2) (packaging may vary)
\tabularnewline 
\hline
\multicolumn{2}{l}{\textbf{Sports}}
\tabularnewline 
\hline
User Interaction History & Here is the visit history list of user: id: 18308 title: Rubbermaid  Shaker Bottle, 20-Ounce, Purple, id: 7317 title: GSI Outdoors Glacier Stainless Steel Plate, id: 17627 title: NOCO Genius GENM2 8 Amp 2-Bank Waterproof Smart On-Board Battery Charger, id: 385 title: Lodge Pro-Logic P12D3 Cast Iron Dutch Oven, Black, 7-Quart, id: 15 title: Lodge Original Finish Pro Grid/Iron Griddle recommend next item
\tabularnewline 
\hline
Next Item & id: 17944 title: Yoga Full Toe Socks (Various Colors), 2 Pairs Value Pack Set
\tabularnewline 
\hline
\multicolumn{2}{l}{\textbf{Toys}}
\tabularnewline 
\hline
User Interaction History & Here is the visit history list of user: id: 188 title: Little Tikes Cozy Coupe, id: 423 title: Music  Lights Sit 'n Spin Rockin' Tunes (colors vary), id: 381 title: Naturally Playful Kangaroo Climber, id: 211 title: Elmo's Rock  Roll Guitar recommend next item
\tabularnewline 
\hline
Next Item & id: 412 title: Turtle Sandbox
\tabularnewline 
\hline 
\end{tabular}
 \caption{Text Representations of Items Used in SREDR. We sample four cases from Yelp, Beauty, Sports, and Toys, to show  the verbalization results of user-item interaction history and items.}
 \label{tab:verbalization}
\end{table*}

\begin{table*}
\small
\centering
\resizebox{\textwidth}{!}{
\begin{tabular}{ l | r r r | r r r | r r r | r r r }
\hline
\multirow{2}{*}{\textbf{Num}} & \multicolumn{3}{c}{\textbf{Beauty}} & \multicolumn{3}{c}{\textbf{Yelp}} & \multicolumn{3}{c}{\textbf{Sports}} & \multicolumn{3}{c}{\textbf{Toys}}  \\ \cline{2-13}
& Train   & Dev & Test & Train   & Dev & Test & Train   & Dev & Test & Train   & Dev & Test\\\hline
>256 & 37,857 & 4,634 & 5,693 & 44,035 & 3,158 & 3,507 & 34,374 & 5,267 & 6,533 & 21,663 & 2,173 & 2,577  \\
>512 & 19,185 & 1,472 & 1,663 & 16,017 & 842 & 911 & 11,728 & 1,165 & 1,335 & 9,384 & 607 & 661  \\
Mean & 276 & 221 & 252 & 164 & 132 & 147 & 172 & 172 & 198 & 183 & 151 & 173  \\
Mid & 129 & 142 & 173 & 92 & 87 & 102 & 100 & 125 & 152 & 93 & 106 & 128  \\
Mode & 40 & 95 & 135 & 25 & 55 & 71 & 34 & 89 & 118 & 31 & 76 & 100  \\
\hline
\end{tabular}}
\caption{Statistics of Text Tokens of User-Item Interaction Sequences.}
\label{tab:token}
\end{table*}

\section{Appendix}

\subsection{More Details of Data Preprocessing}\label{app:datapro}

In this subsection, we describe more details of data preprocessing and the data partition.

We use Recbole~\cite{zhao2021recbole} to process all datasets and show the configurations in Listing~\ref{lst:data}. All experiments keep the same setting as previous work~\cite{Xie2022DIF-SR,Zhou2020s3}. For all datasets, we filter out the items and users that appear less than five times in the whole datasets and treat all user-item interactions as implicit feedback~\cite{Xie2022DIF-SR,chen2018sequential,Sun2019Bert4rec}. For the Yelp dataset, we follow previous work~\cite{Xie2022DIF-SR,Zhou2020s3} and retain user-item interaction records after January 1, 2019. After data processing, each example can be a user-item interaction sequence $\mathcal{H}=\{v_1,v_2,\dots,v_{T} \}$. We also preserve names, addresses and categories of restaurants and product names as item attributes for the items in Yelp dataset  and Amazon Product dataset, respectively. All data statistics on processed datasets are shown in Table~\ref{tab:dataset}.

We follow previous work~\cite{Xie2022DIF-SR}, use the leave-one-out evaluation, and separate the processed datasets into training, development and testing sets. For the user-item interaction sequence $\mathcal{H}=\{v_1,v_2,\dots,v_{T} \}$, we construct the testing and development sets by using previous items $v_{1,...,T-1}$ to predict the last item $v_T$ and using $v_{1,...,T-2}$ to predict the last second item $v_{T-1}$, respectively.
For the training set, we follow~\citet{zhao2021recbole} to use interaction history $v_{1,...,i-1}$ to predict $v_i$ where $ 1<i<T-1$. The statistics of data splits are shown in Table~\ref{tab:split}. This split method is widely used in sequential recommendation work~\cite{chen2018sequential,Sun2019Bert4rec}. Besides data preprocessing, we also use the Recbole~\cite{zhao2021recbole} for data partitioning, which allows us to be consistent with the baseline in data for a fair comparison with our baseline model~\cite{Xie2022DIF-SR}.

\lstset{
    basicstyle=\small,
}
\begin{lstlisting}[language=Python, caption=The Configurations of Dataset Processing using RecBole., label=lst:data]

# Yelp (Data Preprocessing)
val_interval: 
{'date': "[1546264800,1577714400]"}
filter_inter_by_user_or_item: True
user_inter_num_interval: "[5,inf)"
item_inter_num_interval: "[5,inf)"

# Amazon Product (Data Preprocessing)
val_interval:
filter_inter_by_user_or_item: True
user_inter_num_interval: "[5,inf)"
item_inter_num_interval: "[5,inf)"

# Leave-one-out Evaluation (Data Split)
eval_args:
  split: { 'LS': 'valid_and_test' }
  group_by: user
  order: TO
  mode: full
\end{lstlisting}

\subsection{More Details of Evaluation Settings}\label{app:metrics}
We use the leave-one-out evaluation and train SREDR to predict the next item using previously user-interacted items. For all experiments, we keep the same evaluation metrics as DIF-SR~\cite{Xie2022DIF-SR} and choose the same $k$ values.

During evaluating our models, we utilize a full ranking testing scenario, which is the same as DIF-SR~\cite{Xie2022DIF-SR}. Some work evaluates model performance on a small item subset by randomly sampling or sampling items according to item popularity, making the evaluation results inconsistent of the same model. Instead of reranking items in sampled subsets, some work~\cite{krichene2022sampled,dallmann2021case} builds a more realistic recommendation evaluation setting by full reranking items and choose the top-ranked items as recommendation results.

\subsection{Experiment Details of Negative Sampling}\label{app:negative}
We optimize the model using inbatch negatives and negative samples sampled by the corresponding negative sampling method. During the training process, we set batch size=8 and each training sample corresponds to 1 positive sample and 9 negative samples. More specifically, for one batch, 7 (inbatch negatives) plus 72 (9 sampled negatives for each training example) negatives are used for training.

We randomly sample 100 items as random negative samples. Following ~\cite{Sun2019Bert4rec}, we sample popular negatives. We count the frequency of items in the full data set, and sort them from high to low, and retain top 500 as a popular item set, and randomly sample 100 of them as negative samples for each sample. We use the top100 predicted by T5-DPR as hard negatives~\cite{xiong2020approximate}. It is worth noting that when sampling negative samples, we filter out user-interacted items and target items to be predicted for each sample to ensure that they will not be sampled as negative samples.

The model trained by hard negatives starts from the T5-DPR checkpoint which trained by inbatch negatives, we set learning rate=5e-5, warm up proportion=0. And the random negative method and popular negative method are initialized with T5-base checkpoint from huggingface~\cite{wolf2019huggingface}, we set learning rate=1e-4, warm up proportion=0.1. Our experimental results are presented in Table~\ref{tab:ablation}.

\subsection{Text based Item Representations in SREDR}\label{app:text_rep}
SREDR verbalizes the items using item identifiers and attributes. Here we provide some cases in Table~\ref{tab:verbalization} to help readers better understand how SREDR represent the items and user-item interactions.

For user-item interaction sequence representations, we follow P5~\cite{Geng0FGZ22} and use the template ``Here is the visit history list of user: $X(\mathcal{H})$ recommend next item'' to demonstrate the sequential recommendation task, making language models better understand the task. Here $X(\mathcal{H})$ is the concatenation of text representations of historically user-interacted item sequence, which is defined in E.q.~\ref{eq:seqtext}. We reserve the user-item interaction history to satisfy the max length truncation operation of language models. The lengths of text representations of user-item interactions are counted in Table~\ref{tab:token}.

To represent items using text utterances, we use different attributes to verbalize items in Yelp and Amazon product datasets:
\begin{itemize}
\setlength{\itemsep}{0pt}
\setlength{\parsep}{0pt}
\setlength{\parskip}{0pt}
    \item \textbf{Yelp:} We reserve the \textit{names},  \textit{addresses} and  \textit{categories} of restaurants, which is the same as DIF-SR~\cite{Xie2022DIF-SR}.
    \item \textbf{Amazon Beauty:} We found the product attributes are usually described in the names of products. Thus, we only reserve the \textit{names} of products to verbalize items.
\end{itemize}
All attributes of items are concatenated as text representations using E.q.~\ref{eq:item}.

% \input{table/suboverall.tex}
% \subsection{Recommendation Performance of Additional Baseline Models}\label{app:add_exp}

% In Table~\ref{tab:suboverall}, we show more comparison results of baseline models. GRU4Rec~\cite{Hidasi2015session} is one previous baseline, which uses RNN to model user-item interaction sequences for recommendation. ICAI-SR~\cite{yuan2021icai} is compared, which proposes a heterogeneous graph to represent the relations between items and attributes to model item relevance. Besides, NOVA~\cite{Liu2021nova} is also compared, which is similar to DIF-SR and builds attention mechanisms to fuse attributes to model side information. 
% Compared with above models, SREDR shows its effectiveness by outperforming these models.

\begin{table}[t]
\begin{center}
\small

\begin{tabular}{l|c|   c   | c }
\hline 
\textbf{Dataset} & \textbf{Metrics} &  \textbf{DIF-SR}  &  \textbf{SREDR}\\ 
\hline
\multirow{4}{*}{Beauty} & HR@10 & 0.0909 & \textbf{0.1030}  \\
& HR@20  & 0.1278  & \textbf{0.1550}  \\
& MRR@10  & 0.0308 & \textbf{0.0362}  \\
& MRR@20  &0.0333  & \textbf{0.0398}  \\
\hline
\multirow{4}{*}{Sports} & HR@10 & 0.0540 & \textbf{0.0633}  \\
& HR@20  & 0.0783  & \textbf{0.0964}  \\
& MRR@10  & 0.0162 & \textbf{0.0248}  \\
& MRR@20  &0.0178  & \textbf{0.0271}  \\
\hline
\multirow{4}{*}{Toys} & HR@10 & 0.0953 & \textbf{0.1232}  \\
& HR@20  & 0.1343  & \textbf{0.1789}  \\
& MRR@10  & 0.0320 & \textbf{0.0460}  \\
& MRR@20  &0.0347  & \textbf{0.0498}  \\
\hline
\multirow{4}{*}{Yelp} & HR@10 & 0.0681 & \textbf{0.0738}  \\
& HR@20  & 0.0985  & \textbf{0.1156}  \\
& MRR@10  & \textbf{0.0331} & 0.0294  \\
& MRR@20  & \textbf{0.0351}  & 0.0322  \\
\hline
\end{tabular}
\end{center}
\caption{\label{tab:appeval} Additional Evaluations for Recommendation Effectiveness of SREDR. We use two additional evaluation metrics, Hit-Ratio and MRR, to evaluate the performance of SREDR and our main baseline model, DIF-SR~\cite{Xie2022DIF-SR}.}

\end{table}
\subsection{SREDR Evaluations using More Metrics}\label{app:add_eval}
As shown in Table~\ref{tab:appeval}, we also conduct additional experiments to evaluate the recommendation effectiveness of SREDR using MRR and Hit Ratio. SREDR usually shows its advance by outperforming previous state-of-the-art model, DIF-SR. SREDR shows less effectiveness on ranking appropriate restaurants more ahead, which may lies in that the embedding based recommendation methods has the ability to model some implicit user characteristics and user-item dependencies.

\begin{table}
\centering
\resizebox{0.48\textwidth}{!}{
\begin{tabular}{ l | c  |  c | c | c | c  }
\hline
\multirow{2}{*}{\textbf{Datasets}} & \multirow{2}{*}{\textbf{\#Threshold}} & \multicolumn{2}{c|}{\textbf{Low Frequency}} & \multicolumn{2}{c}{\textbf{High Frequency}} \\ \cline{3-6}
& & \#Item   & \#Sample   & \#Item   & \#Sample \\
\hline
Beauty & 16 & 6365 & 13767 & 1613 & 8596  \\
Yelp & 19 & 10207 & 17756 & 2723 & 12743  \\
Sports & 16 & 10073 & 21831 & 2521 & 13767  \\
Toys & 15 & 5924 & 12718 & 1551 & 6694  \\
\hline
\end{tabular}}
\caption{Data Statistics with Different User Interacted Frequencies. We set the threshold according to the ratio of 8:2~\cite{ZhihongChen2020ESAMDD} to divide the label items in the test set into low-frequency items and high-frequency items. We split the testing datasets into two groups, low frequency and higher frequency, according to the user interacted frequency of items.}
\label{tab:freq}
\end{table}
\subsection{More Experiments on Items with Different User Interacted Frequencies}\label{app:freq}

Our experiments divide the items into low-frequent and higher-frequent groups according to user interacted frequencies, aiming to explore the cold start problem in representing items, which is a well-known problem in recommendation systems~\cite{pan2019warm,YongchunZhu2021LearningTW}.
To calculate the user-interacted frequency of predicted items in the test set, we first count the frequency of items appearing as predicted labels in the training, as well as, we set the frequency of items that do not appear in predicted labels as 0. Then we sort the items according to the user-interacted frequency and set the thresholds of user-interacted frequency to separate the items into low-frequent and high-frequency groups.

As shown in Sec.~\ref{sec:scenarios}, the user-interacted frequency thresholds are set to 15, 16 and 19 to approximately keep the ratio of higher-frequent items and low-frequent items as 8:2. Such a participation is come from the Pareto principle (80/20 rule) and previous recommendation work also uses such a ratio to define the long tail items~\cite{ZhihongChen2020ESAMDD}. All data statistics are shown in the Table~\ref{tab:freq}. Even though SREDR has shown strong effectiveness on generalizing low-frequent items (Figure~\ref{fig:freq}), we conduct additional experiments by setting different thresholds of user-interacted frequency to avoid the bias from item partition. 

Furthermore, we set the user-interacted frequencies to approximately keep the ratios of low-frequent items being from 10\% to 90\%. We show the recommendation performance of SREDR and T5 in Figure~\ref{fig:ratio}, which are text-based and embedding-based recommendation models. T5 indeed shows slightly improvements on very frequently interacted items by learning embedding to establish latent dependencies among items. Nevertheless, such an embedding based recommendation modeling method can not be easily generalized to low-frequent items. Notably, SREDR shows consist improvements over T5, which confirms that fully text based modeling methods can alleviate the cold start problem~\cite{lam2008addressing,schein2002methods} during learning representations of low-frequent items.

\input{figure/ratio}

\begin{table*}
\small
\centering
\resizebox{\textwidth}{!}{
\begin{tabular}{l|c| c|  c  c   c  c  |  c  }
\hline 
\multirow{2}{*}{\textbf{Dataset}} & \multirow{2}{*}{\textbf{Metrics}} &  \textbf{T5-DPR w/o Prompt} &  \multicolumn{4}{c|}{\textbf{T5-DPR}} & \textbf{T5-DPR (Rand Negs)} \\
& &\textbf{(Inbatch)} & \textbf{Inbatch}  & \textbf{Popular Negs}  & \textbf{Hard Negs} & \textbf{Random Negs} & \textbf{w/ Longer History} \\ 
\hline
\multirow{4}{*}{Yelp} & Recall@10 & 0.0441 &  0.0460  &0.0351 & 0.0324 & 0.0726& \textbf{0.0733}  \\
& Recall@20  & 0.0714  & 0.0740 & 0.0550 & 0.0519 & 0.1131& \textbf{0.1150}  \\
& NDCG@10  & 0.0235 & 0.0250 & 0.0186& 0.0173 & 0.0388& \textbf{0.0393}  \\
& NDCG@20  &0.0304  & 0.0320 & 0.0236 & 0.0222 & 0.0489& \textbf{0.0498}  \\
\hline
\multirow{4}{*}{Sports} & Recall@10   &0.0327 &0.0329 & 0.0284 & 0.0354 & 0.0510& \textbf{0.0545} \\
& Recall@20 &0.0550 &0.0554 &0.0476 & 0.0550 & 0.0812& \textbf{0.0851} \\
& NDCG@10  &0.0155 &0.0159 &0.0135 & 0.0182 & 0.0249& 
 \textbf{0.0270}  \\
& NDCG@20 &0.0211 &0.0216 & 0.0184 & 0.0232 & 0.0325& \textbf{0.0346}  \\
\hline
\multirow{4}{*}{Beauty} & Recall@10  & 0.0688 & 0.0716 &  0.0601  &0.0750 & 0.0921 & \textbf{0.0935} \\
& Recall@20  & 0.1088  & 0.1082 & 0.0950 & 0.1147 & 0.1401& \textbf{0.1441} \\
& NDCG@10 & 0.0335 & 0.0345 & 0.0294  & 0.0368 & 0.0444& \textbf{0.0445} \\
& NDCG@20 &0.0435  & 0.0437 & 0.0382 & 0.0468 & 0.0565& \textbf{0.0573} \\
\hline
\multirow{4}{*}{Toys} & Recall@10  & 0.0777 &  0.0805  &0.0678  & 0.0878 & 0.1032& \textbf{0.1056} \\
& Recall@20 & 0.1222  & 0.1243 & 0.1065 & 0.1297 & 0.1577& \textbf{0.1594} \\
& NDCG@10  & 0.0369 & 0.0375 & 0.0326 & 0.0426 & 0.0488& \textbf{0.0508}  \\
& NDCG@20 &0.0480  & 0.0485 & 0.0423 & 0.0532 & 0.0625& \textbf{0.0643} \\
 \hline

\end{tabular}}
\caption{\label{tab:comablation}More Experimental Results of Ablation Study.}

\end{table*}
\subsection{More Evaluation Results of Ablation Study of SREDR}\label{app:ablation}
As shown in Table~\ref{tab:comablation}, we show complete evaluation results of Sec.~\ref{sec:ablation}. Our experiments illustrate that the designed modules of SREDR indeed plays important roles in conducting more accurate recommendation results.

The template-based prompt learning method and longer user-item interaction modeling method help language models better represent the user intentions by demonstrating the recommendation task and capture more semantics from longer user-item interaction sequences. Besides, more experimental results further showcase that the random sampled negatives are suitable to train recommendation systems among all negative sampling methods.

\subsection{License}
We show the licenses of the datasets that we use. Yelp uses Apache License 2.0, while Amazon Product shows its terms of use at website\footnote{\url{http://jmcauley.ucsd.edu/data/amazon/}}. All of these licenses and agreements allow their data for academic use.

\end{appendix}
